# Supplementary material for: Persistence of Island Arrangements During Layer-by-Layer Growth Revealed Using Coherent X-rays
Source: arXiv:1804.08161 ancillary file (2018-04-22)
Supplement: Supplementary file 1 [file 2018_GJu_TwoTime_m_plane_XPCS_Supplemental_v1.pdf]

# Supplementary Information for "Persistence of Island Arrangements During Layer-by-Layer Growth Revealed Using Coherent X-rays"


Guangxu Ju,[1] Dongwei Xu,[1,*] Matthew J. Highland,[1] Carol Thompson,[2] Hua Zhou,[3] Jeffrey A. Eastman,[1] Paul H. Fuoss,[1,†] Peter Zapol,[1] Hyunjung Kim,[4] and G. Brian Stephenson[1,‡]

[1]*Materials Science Division, Argonne National Laboratory, Argonne, IL 60439 USA*

[2]*Department of Physics, Northern Illinois University, DeKalb IL 60115 USA*

[3]*X-ray Science Division, Argonne National Laboratory, Argonne, IL 60439 USA*

[4]*Department of Physics, Sogang University, Seoul, 04107 Korea*



(Dated: April 22, 2018)


## S1. X-RAY OPTICS AND DETECTOR FOR PINK BEAM XPCS

The undulator spectrum has peaks at all harmonic multiples of the fundamental energy. We used the 3rd harmonic at 25.75 keV. A compound refractive lens (CRL) was used to focus the beam vertically[1]. It consisted of a set of 42 individual double-concave Be lenses with 200 $\mu$m tip radii (obtained from RXOPTICS, Monschau, Germany), that was installed at a distance $L_s = 67.40$ m from the source and $L_d = 4.97$ m from the sample. A water-cooled aperture with 100 $\mu$m vertical size was placed in front of the CRL to reduce heat load and select the vertical coherent fraction. An 8 m length of flight path filled with nitrogen at 1 atm was used to absorb most of the 1st and 2nd harmonics upstream of the water-cooled aperture. The 25.75 keV energy was the highest that the CRL would focus, chosen to minimize interaction of the x-ray beam with the growth process, which we observed for focused pink beam at 10 keV.

It was also important to reduce the intensity of the higher harmonics, since the $(1\,0\,\overline{1}\,0)$ Bragg peaks for the 4th, 5th, 6th, and higher harmonics occur along the specular CTR $(H\,0\,\overline{H}\,0)$ at $H = 3/4, 3/5, 3/6$ etc., contaminating the scattering signal from the surface. While the first optical element on the beamline, a mirror with a critical energy of 30 keV, helps to remove the higher harmonics, we found it necessary to install an additional double-bounce mirror pair to reduce their contribution further. These were adjusted to place their critical energy just above the 25.75 keV energy used. The chromaticity of the CRL also helps to reject unwanted harmonics, since they do not focus at the same distance. A vertical slit of 10 $\mu$m width 150 mm upstream of the sample served as an order-sorting aperture to reject unfocused harmonics. Because a small peak from the 6th harmonic could still be observed on the CTR at the anti-Bragg position ($H = 0.5$), we recorded data at $H = 0.48$ to avoid the harmonic contamination.

The GaAs sensor of the detector had a non-uniform pixel-to-pixel response. We characterized this response by collecting long integrations of uniform scattering from a standard glass sample to obtain a "flatfield" pattern. The measured scattering patterns were divided by this flatfield response, as well as normalized to an incident intensity monitor just upstream of the sample. Several percent of the detector pixels were non-functional, and these were removed prior to carrying out the speckle analysis. These "bad" pixels were identified as those having a flatfield response less then 40% or more than 200% of the average.

## S2. HILLOCK MORPHOLOGY

Analysis of the scattering patterns in reciprocal space provides a quantitative understanding of the sample surface morphology. Since GaN has a hexagonal crystal structure, it is convenient to use both orthonormal coordinates $Q_X$, $Q_Y$, and $Q_Z$ in Å$^{-1}$, as well as the standard hexagonal Miller-Bravais indices $(H\,K\,I\,L)$ in reciprocal lattice units. The reciprocal space direction normal to the m-plane surface is $(1\,0\,\overline{1}\,0)$, which we denote as $Q_Y$. The two perpendicular in-plane directions are $(1\,\overline{2}\,1\,0)$ and $(0\,0\,0\,1)$, which we denote as $Q_X$ and $Q_Z$. The lattice parameters in the corresponding $x$ and $z$ in-plane directions are $a = 3.188$ and $c = 5.185$ Å, respectively. The monolayer spacing in the surface normal $y$ direction is $\sqrt{3}a/2 = 2.761$ Å. The positions of the $(1\,0\,\overline{1}\,0)$, $(1\,\overline{2}\,1\,0)$, and $(0\,0\,0\,1)$ Bragg peaks correspond to $Q_X = 2\pi/a = 1.97$ Å$^{-1}$, $Q_Y = 4\pi/\sqrt{3}a = 2.28$ Å$^{-1}$, and $Q_Z = 2\pi/c = 1.21$ Å$^{-1}$, respectively.

The reciprocal space area covered by the pixels of the area detector, at the $H = 0.48$ ($Q_Y = 1.09$ Å$^{-1}$) position used in the growth studies, forms a slightly spherically curved surface inclined at an angle $\theta = 2.4°$ from the surface normal (Fig. S1 (a)). Because speckle and other diffraction features from the surface are extended in the $Q_Y$ surface normal direction, the scattering pattern on the detector can simply be projected into the surface plane to characterize the in-plane surface morphology. The square detector area thus projects into a rectangular strip in the $Q_X$-$Q_Z$ plane (Fig. S1 (b)). We chose a sample orientation so that the diffuse scattering from the anisotropic islands, extended in the $Q_Z$ direction, is covered by this strip.

During growth on low-miscut m-plane GaN, an initially flat surface has been found to be unstable with respect to the formation of shallow faceted hillocks, due to spiral growth around threading dislocations with a screw component[2]. These hillocks have a size and spacing that depends upon threading dislocation density, and a typical facet slope of less than 1 degree. In this work, we observed such a hillock morphology on our samples, as evidenced by the multiple crystal truncation rods (CTRs) from the hillock facet surface normals. Atomic force microscopy showed that the typical hillock size and spacing was $10 \times 40$ $\mu$m on our sample.

The observed CTRs corresponded with different facets of the hillocks (Fig. S1 (b)). The miscut of facet 1 away from the $(1\,0\,\overline{1}\,0)$ m-plane was typically $\sim 0.32°$, while the miscut of facets 2 and 4 was $\sim 0.09°$. Facet 3 had a higher miscut and we typically did not observe a CTR from it. During growth, the diffuse scattering observed at high $Q_Z$ arose primarily from islands aligned with the terraces on facet 1 of the hillocks.

## S3. SPECKLE ANALYSIS, CONTRAST, AND STABILITY

Analysis of two-time correlations in XPCS from non-steady-state systems can be a challenge, since the mean intensity $\overline{I}(\mathbf{Q}, t)$ that provides the reference level for the speckle $\Delta I$ is a function of time and thus cannot be obtained simply by averaging in time. We explored a method to obtain $\overline{I}(\mathbf{Q}, t)$ by smoothing $I(\mathbf{Q}, t)$ over neighboring pixels. A Savitzky-Golay smoothing[3] was applied using pixel ranges optimized for the dataset at each $T$ (values in Table S1). We found that, if the pixel range is too large, $\mathbf{Q}$ dependence in the mean intensity will be smoothed away, leading to an overestimate of $\Delta I$, while if the pixel range is too small, the smoothed function will include some of the contrast from speckle and counting statistics, leading to an underestimate of $\Delta I$. The optimum smoothing pixel range changes with $T$

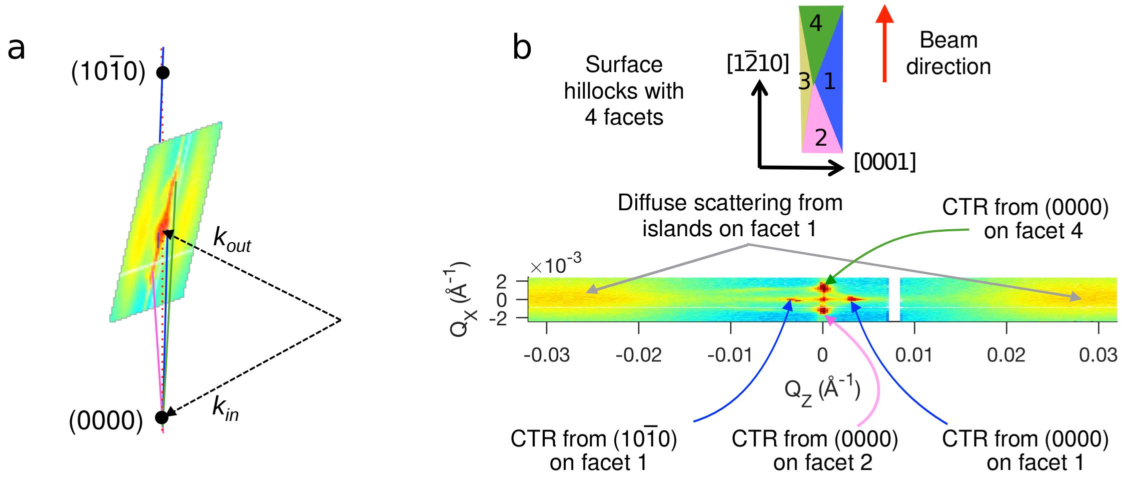


FIG. S1. **Detector, hillock, and CTR orientations.** **a**, Orientation of detector in reciprocal space. **b**, Hillock surface morphology and correspondence with observed crystal truncation rods (CTRs).

TABLE S1. **Parameters used in speckle analysis.** For the dataset at each temperature, we list the number of pixels $i$ and $j$ in the moving window used for smoothing in the $Q_X$ and $Q_Z$ directions, respectively, and the $Q_X$ and $Q_Z$ ranges for ensemble averages to follow the diffuse scattering maxima at $\pm Q_Z^{max}$.

| Temperature (K) | $i$ | $j$ | $Q_X$ Å$^{-1}$ | $Q_Z$ Å$^{-1}$ | $Q_Z^{max}$ Å$^{-1}$ |
|---|---|---|---|---|---|
| 914 | 11 | 3 | $\|Q_Y\| \leq 0.0004$ | $0.0057 \leq \|Q_Z\| \leq 0.0099$ | 0.0060 |
| 891 | 11 | 5 | $\|Q_Y\| \leq 0.0005$ | $0.0057 \leq \|Q_Z\| \leq 0.0141$ | 0.0084 |
| 867 | 11 | 5 | $\|Q_Y\| \leq 0.0008$ | $0.0075 \leq \|Q_Z\| \leq 0.0186$ | 0.0111 |
| 843 | 11 | 7 | $\|Q_Y\| \leq 0.0009$ | $0.0099 \leq \|Q_Z\| \leq 0.0246$ | 0.0147 |
| 820 | 11 | 7 | $\|Q_Y\| \leq 0.0010$ | $0.0129 \leq \|Q_Z\| \leq 0.0321$ | 0.0192 |
| 796 | 11 | 9 | $\|Q_Y\| \leq 0.0011$ | $0.0168 \leq \|Q_Z\| \leq 0.042$ | 0.0252 |
| 772 | 11 | 9 | $\|Q_Y\| \leq 0.0013$ | $0.0222 \leq \|Q_Z\| \leq 0.0553$ | 0.0333 |
| 747 | 11 | 11 | $\|Q_Y\| \leq 0.0015$ | $0.0255 \leq \|Q_Z\| \leq 0.0637$ | 0.0381 |

because of the variation in the sharpness of the mean intensity in $\mathbf{Q}$, and the proximity of the CTRs to the diffuse scattering. For each $T$ we found a region of pixel ranges where the result for $\Delta I$ did not depend sensitively on the choice.

Likewise, the region of $\mathbf{Q}$ used to obtain the ensemble average $\langle\rangle$ in equation (1) of the main paper was varied with $T$ to follow the region of intense diffuse scattering (values in Table S1).

To optimize the experimental conditions, the $\mathbf{Q}$ resolution is purposely set to be less than that required to give 100% contrast, in order to increase the signal and reduce noise in the correlation function arising from counting statistics. As a check on the accuracy of the smoothing method described above to separate speckle $\Delta I$ from variations in the mean intensity $\bar{I}$, we can compare the observed speckle contrast to that expected based on the

experimental conditions.

The distribution of intensity $I$ in a continuous speckle pattern with $M$ modes is described by the Gamma distribution,

$$P_\Gamma(I) = \frac{M^M I^{M-1}}{\Gamma(M)\overline{I}^M} \exp(-MI/I), \tag{S1}$$

where the mean of this distribution is $\overline{I}$ and the contrast (variance divided by the square of the mean, $\mathrm{Var}_\Gamma/\overline{I}^2$) is equal to $M^{-1}$. The contrast can be extracted from intense speckle patterns by evaluating the experimental variance and mean in the signal distribution on the detector[4–6]. For weak speckle patterns, the fluctuations due to photon counting statistics (shot noise) must be considered[4,7,8]. The probability distribution for the number of photons per pixel $k$ in a discrete speckle pattern is described by the negative binomial distribution,[7] which is the convolution of the Gamma and Poisson distributions,

$$P_{NB}(k) = \frac{\Gamma(k+M)}{\Gamma(M)\Gamma(k+1)} \left(1 + \frac{M}{\overline{k}}\right)^{-k} \left(1 + \frac{\overline{k}}{M}\right)^{-M}. \tag{S2}$$

Here the mean number of photons per pixel in the discrete speckle pattern is $\overline{k}$ and the contrast is the sum of those for the Gamma and the Poisson distributions, $\mathrm{Var}_{NB}/\overline{k}^2 = M^{-1} + \overline{k}^{-1}$. For weak speckle patterns, e.g. $\overline{k} < 1$, the extra term $\overline{k}^{-1}$ from photon counting statistics is larger than the speckle contrast term $M^{-1}$.

Our two-time correlation function is constructed so that the equal-time $\Delta t = 0$ points along the diagonal give an experimental measure of the contrast. We can correct these diagonal values by subtracting the known Poisson shot noise term $\overline{k}^{-1}$ to obtain the speckle contrast $M^{-1}$ (Fig. S2). While the value of $\overline{k}$ can be small at lower $T$ (e.g. 5 counts per 30 s at 796 K) and thus the Poisson term large, when the time-dependent Poisson term is subtracted, the remaining speckle contrast term is relatively independent of time, in agreement with expectations. We have performed this extraction of the speckle contrast for each $T$, and we find that the mean speckle contrast is about 1% in each case (Fig. S3). We can also obtain an estimate of the speckle contrast directly from the correlation function values with the smallest non-zero-value of $\Delta t = 0.04$ ML that lie next to the diagonal, since the shot noise is uncorrelated at the two times and does not contribute. The means of these values agree well with those of the shot-noise-corrected diagonal values (Fig. S3).

The speckle contrast expected from the experimental conditions can be estimated by comparing the resolution in reciprocal space to that required to fully resolve the speckle. The shape of a "speckle" (i.e. signal correlation volume) in reciprocal space can be calculated from the shape of the scattering volume in real space. For speckle arising from surface features, the relevant resolution directions in reciprocal space are the in-plane directions $Q_X$ and $Q_Z$. The experimental resolutions can be expressed as

$$\delta Q_X^{exp} = \left[ (kr_v \sin\theta)^2 + (kr_{det} \sin\theta)^2 + \left(\frac{\Delta E}{E} Q_X\right)^2 \right]^{1/2}, \tag{S3}$$

$$\delta Q_Z^{exp} = \left[ (kr_h)^2 + (kr_{det})^2 + \left(\frac{\Delta E}{E} Q_Z\right)^2 \right]^{1/2}, \tag{S4}$$

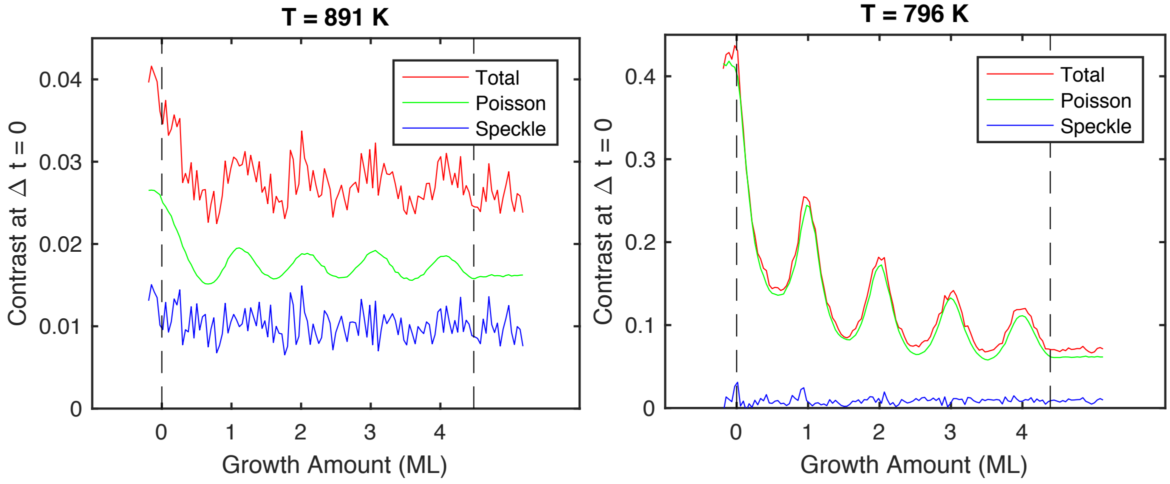


FIG. S2. **Contrast at $\Delta t = 0$.** Data are for two typical temperatures. Contribution from speckle is obtained by subtracting that from Poisson photon counting statistics (self-correlated shot noise).

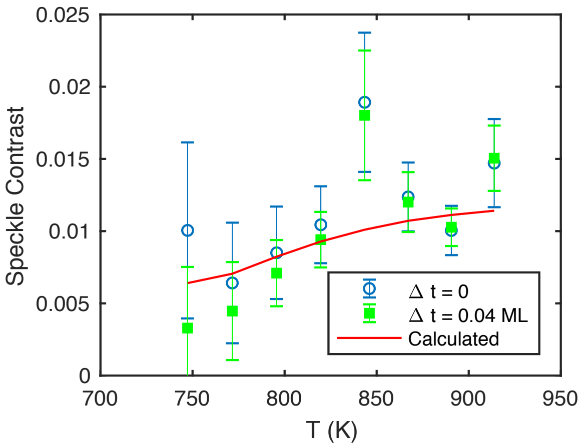


FIG. S3. **Speckle contrast as a function of temperature.** Observed values are averaged over times beyond the first ML of growth, for $\Delta t = 0$ and 0.04 ML. Also shown (curve) is calculation based on experimental parameters. The decreased contrast at lower $T$ is due to the effect of the energy bandwidth of the pink beam as the scattering moves to higher $Q_Z$.

where $k = 2\pi/\lambda$ is the x-ray wavenumber, $\theta = 2.4°$ is the Bragg angle, $r_v = 2.0 \times 10^{-5}$ and $r_h = 0.9 \times 10^{-5}$ are the vertical and horizontal angular divergences (FWHM) incident on the sample, $r_{det} = 2.3 \times 10^{-5}$ is the angular resolution of the detector, and the third terms are the effect of the energy bandwidth $\Delta E/E = 1.3 \times 10^{-2}$. Because the surface speckle are extended in the $Q_Y$ direction, only the in-plane components of the poor radial resolution due to the large bandwidth of the pink beam affect the speckle contrast (Fig. S4). The in-plane extents of the speckle are related to the incident vertical and horizontal beam sizes $w_v = 4$ and $w_h = 16$ $\mu$m by

$$\delta Q_X^{sp} = \pi \sin\theta / w_v, \tag{S5}$$

$$\delta Q_Z^{sp} = \pi / w_h. \tag{S6}$$

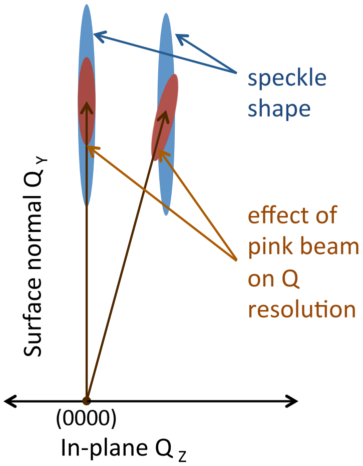


FIG. S4. **Effect of pink beam on speckle contrast.** Speckles from 2D surface features are greatly extended in the surface normal ($Q_Y$) direction. On the specular CTR ($Q_Z = Q_X = 0$), the poor radial resolution due to the wide energy bandwidth of the pink beam aligns with the extended direction of the speckle, and has no effect on observed speckle contrast. The reduction in contrast from surface speckle using pink beam is proportional to the in-plane components $Q_Z$ and $Q_X$, and is independent of $Q_Y$. Thus XPCS studies of atomic-scale surface features at large $Q_Y$ and small $Q_Z$, $Q_X$ can take advantage of the high transverse coherent flux in the pink beam.

The speckle contrast can be written as

$$C_{sp} = \left[1 + \left(\frac{\delta Q_X^{exp}}{\delta Q_X^{sp}}\right)^2\right]^{-1/2} \left[1 + \left(\frac{\delta Q_Z^{exp}}{\delta Q_Z^{sp}}\right)^2\right]^{-1/2}. \tag{S7}$$

In the limit of $r_{det} = 0$ and $\Delta E/E = 0$, this reduces to

$$C_{sp} = \left[1 + \left(\frac{w_v}{\xi_v}\right)^2\right]^{-1/2} \left[1 + \left(\frac{w_h}{\xi_h}\right)^2\right]^{-1/2}, \tag{S8}$$

where $\xi_v \equiv \lambda/(2r_v)$ and $\xi_h \equiv \lambda/(2r_h)$ are the transverse coherence lengths in the vertical and horizontal directions, respectively.

Using the $Q_Z$ value of the center of the diffuse scattering at each temperature, and $Q_X = 0$, the estimated speckle contrast is plotted as a curve along with the observed speckle contrast in Fig. S3. We see that both the expected contrast value at zero $Q_Z$ (1.2 %) and the decrease in contrast as the diffuse scattering moves to higher $Q_Z$ at lower $T$ are generally in agreement with the experimental values. The experimental value at 843 K is significantly higher than that expected, perhaps due to some extra sharp scattering feature in the **Q** window from the surface region studied at this $T$. The good agreement between the measured and calculated speckle contrast provides some assurance that the experimental setup with pink beam and analysis method developed are yielding two-time correlations that reflect the surface dynamics of the sample.

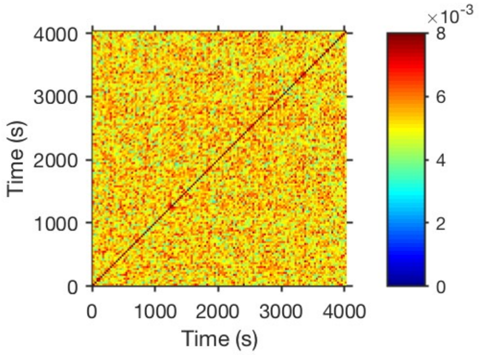


FIG. S5. **Demonstration of stability.** Two-time correlation of a sample held at $T = 796$ K with no growth, after deposition of 4.5 ML. The uniform correlation indicates that the illuminated area is stable over the typical 4000 s time period of our measurements, and that the island structure formed during growth does not continue to evolve after growth under these conditions.

A major challenge in performing an *in situ* XPCS study of growth is to maintain the required stability of the sample at high temperature so that the incident beam illuminates the same area during the growth process. We characterized the stability of the experimental setup by measuring the speckle pattern from the sample with no growth at $T = 796$ K, over a similar time period as used in the growth studies, and performing our standard two-time correlation analysis (Fig. S5). The speckle contrast is independent of $\Delta t$, indicating that the experimental setup and illuminated area are stable for time periods longer than our measurements.

## S4. KINETIC MONTE CARLO SIMULATIONS

We used a kinetic Monte Carlo (KMC) model developed to investigate homoepitaxy on various crystal faces of GaN that has been found agree well with observed growth behavior on the m-plane surface[9]. It was not possible to perform the KMC simulation on a system as large as that investigated experimentally; the practical size limit in the simulations, $128 \times 80$ unit cells in the $a$ and $c$ directions, respectively, corresponds to an area of only about 40 nm square. To model the behavior of the island nucleation arrangement of the terraces, we chose the maximum terrace width possible ($W = 40c = 20.7$ nm) and growth conditions that would give an island spacing of $S = 3.2$ nm, corresponding to about $W/S = 6.5$ islands per terrace. Using the NNN model[9], this was a temperature $T/T_0 = 0.25$ and growth rate of $2.0\times10^{-5}$ ML/unit time. Based on the estimated value $T_0 = 3275$ K for GaN[9], this corresponds to a temperature of roughly $T = 818$ K. These values of $T$ and $W/S$ are similar to those in the experiments (Table S2 below).

## S5. TEMPERATURE DEPENDENCE OF TWO-TIME CORRELATIONS

We obtained two-time correlations functions, as defined in equation (1) of the main paper, for growth at eight temperatures $T$ (Fig. S6). The flow rate of the Ga precursor was the same

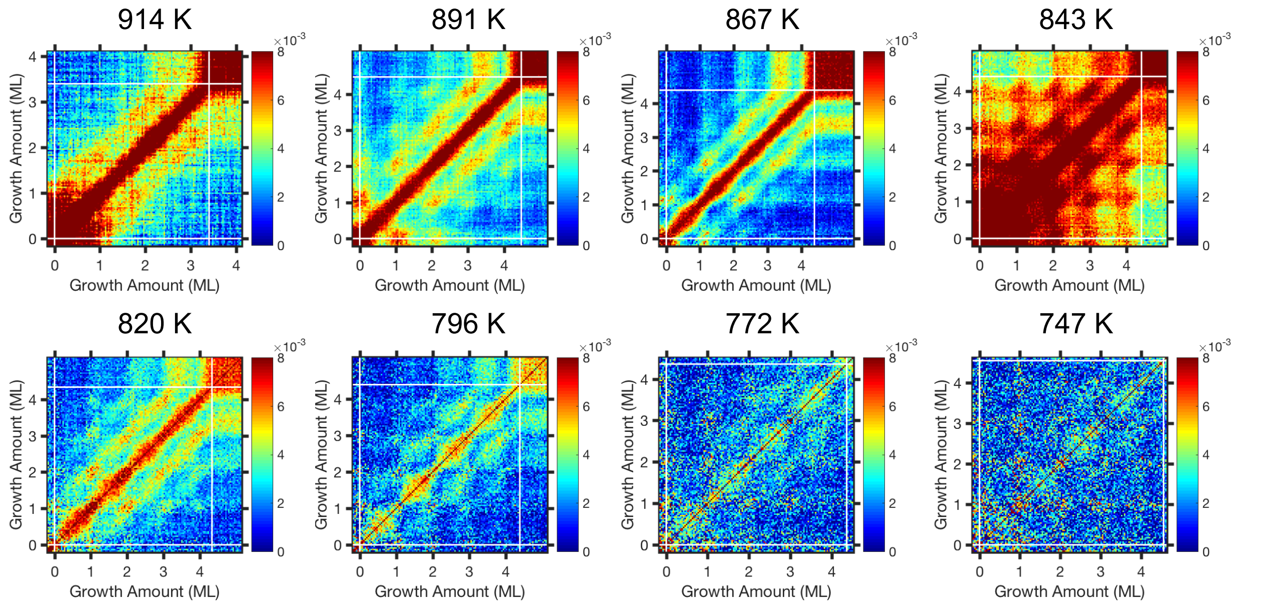


FIG. S6. **Measured two-time correlations.** Plots of $C(t_1, t_2)$ extracted from the measured speckle from 2D islands as a function of growth temperature. Times are expressed as growth amounts in ML.

TABLE S2. **Growth and fit parameters.** Oscillation period of the diffuse scattering, terrace width $W$ on facet 1, island spacing $S$ at 2.5 ML, and number of islands per terrace $W/S$, as well as parameter values providing best fit of $P(\Delta t)$ to equation (S9), for all growth temperatures $T$. The region of the sample surface investigated at the 3 highest $T$ had a smaller terrace width than that at lower $T$.

| Temp. $T$ (K) | Period (s/ML) | Terr. width $W$ (Å) | Isl. spacing $S$ (Å) | $W/S$ | $P_0$ | $A_0$ | $\tau_0$ (ML) | $A^*$ | $\tau^*$ (ML) | $\Delta t_0$ (ML) |
|---|---|---|---|---|---|---|---|---|---|---|
| 914 | 953 | 835 | 1045 | 0.8 | -0.0014 | 0.0078 | 1.17 | 0.0026 | 0.55 | -0.03 |
| 891 | 755 | 835 | 746 | 1.1 | -0.0013 | 0.0051 | 2.03 | 0.0028 | 0.79 | -0.12 |
| 867 | 708 | 835 | 565 | 1.5 | -0.0003 | 0.0053 | 1.91 | 0.0027 | 0.97 | -0.11 |
| 843 | 753 | 1100 | 427 | 2.6 | -0.0035 | 0.0065 | 2.50 | 0.0015 | 1.67 | -0.05 |
| 820 | 761 | 1100 | 327 | 3.4 | -0.0003 | 0.0054 | 2.48 | 0.0015 | 1.56 | -0.07 |
| 796 | 763 | 1100 | 249 | 4.4 | -0.0006 | 0.0034 | 1.92 | 0.0012 | 1.40 | -0.06 |
| 772 | 867 | 1100 | 190 | 5.8 | 0.0000 | 0.0030 | 3.26 | 0.0007 | 2.29 | -0.06 |
| 747 | 846 | 1100 | 165 | 6.7 | -0.0012 | 0.0014 | 1.61 | 0.0005 | 1.74 | -0.08 |

for all growths, resulting in approximately the same growth rate of $1.25 \pm 0.2 \times 10^{-3}$ ML/s as monitored by the period of the oscillations in the diffuse intensity (Table S2). During growth, all except the 914 K data near the step-flow boundary showed "checkerboard" patterns with periods of 1 ML, indicating correlations between island arrangements formed on subsequent layers. Before and after growth, the two-time correlations indicate a relatively static speckle pattern. To characterize the persistence of the correlations, we extracted the quantity $P(\Delta t)$ defined in equation (2) of the main paper for each temperature (Fig. S7).

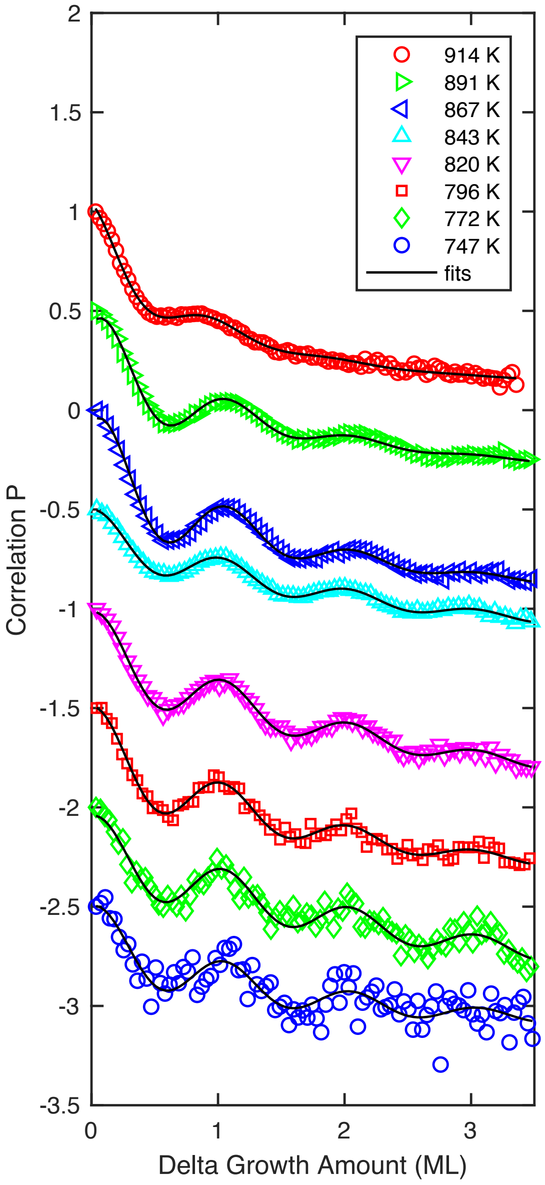


FIG. S7. **Oscillating correlations.** Correlation $P(\Delta t)$ at each temperature and fits to equation (S9). Curves are offset by -0.5 for clarity.

These experimental $P(\Delta t)$ datasets were fit using a non-linear least squares method to an expression of the form

$$P(\Delta t) = P_0 + A_0 \exp(-\Delta t/\tau_0) + A^* \exp(-\Delta t/\tau^*) \cos(2\pi(\Delta t + \Delta t_0)), \quad \text{(S9)}$$

with six fit parameters: $P_0$ is a constant, $A_0$ is the average decay amplitude, $\tau_0$ is the average decay constant, $A^*$ is the amplitude of the oscillating component, $\tau^*$ is the decay constant of the oscillation, and $\Delta t_0$ is the time delay of the oscillation. The fits are shown in Fig. S7, and the best-fit parameter values in Table S2.

## ACKNOWLEDGMENTS

We thank Mark Sutton for suggesting the smoothing method used in the speckle analysis, and Dmitry Byelov of ASI and Russell Woods of the APS Detector Pool for expert assistance with the area detector. Support provided by the Department of Energy, Office of Science, Basic Energy Sciences, Materials Sciences and Engineering (XPCS measurements and analysis) and Scientific User Facilities (KMC model development). Measurements were carried out at the Advanced Photon Source, a DOE Office of Science user facility operated by Argonne National Laboratory. Computing resources were provided on Blues and Fusion, high-performance computing clusters operated by the Laboratory Computing Resource Center at Argonne National Laboratory.

---

* current address: School of Energy and Power Engineering, Huazhong University of Science and Technology, Wuhan 430074, China

† current address: SLAC National Accelerator Laboratory, Menlo Park, CA 94025 USA

‡ correspondence to: stephenson@anl.gov

[1] Guangxu Ju, Matthew J. Highland, Carol Thompson, Jeffrey A. Eastman, Paul H. Fuoss, Hua Zhou, Roger Dejus, and G. Brian Stephenson, "Characterization of the x-ray coherence properties of an undulator beamline at the Advanced Photon Source," Preprint at https://arxiv.org/abs/1802.05675 (2018).

[2] R. M. Farrell, D. A. Haeger, X Chen, C. S. Gallinat, R. W. Davis, M. Cornish, K. Fujito, S. Keller, S. P. DenBaars, S. Nakamura, and J. S. Speck, "Origin of pyramidal hillocks on GaN thin films grown on free-standing m-plane GaN substrates," Applied Physics Letters **96**, 231907 (2010).

[3] Abraham Savitzky and Marcel J. E. Golay, "Smoothing and differentiation of data by simplified least squares procedures." Analytical Chemistry **36**, 1627–1639 (1964).

[4] C Gutt, L-M Stadler, A Duri, T Autenrieth, O Leupold, Y Chushkin, and G Grübel, "Measuring temporal speckle correlations at ultrafast x-ray sources," Optics Express **17**, 55–61 (2009).

[5] C. Gutt, P. Wochner, B. Fischer, H. Conrad, M. Castro-Colin, S. Lee, F. Lehmkühler, I. Steinke, W. Sprung, M .and Roseker, D. Zhu, H. Lemke, S. Bogle, P. H. Fuoss, G. B. Stephenson, M. Cammarata, D. M. Fritz, A. Robert, and G. Grübel, "Single shot spatial and temporal coherence properties of the SLAC linac coherent light source in the hard x-ray regime," Physical Review Letters **108**, 024801 (2012).

[6] Karl F. Ludwig, "X-ray photon correlation spectroscopy in systems without long-range order: existence of an intermediate-field regime," Journal of Synchrotron Radiation **19**, 66–73 (2012).

[7] Joseph W. Goodman, *Speckle phenomena in optics: theory and applications* (Roberts & Company Publishers, 2007) roberts and Company was acquired by Macmillan Learning in 2016.

[8] Frédéric Livet, "Diffraction with a coherent x-ray beam: dynamics and imaging," Acta Crystallographica Section A: Foundations of Crystallography **63**, 87–107 (2007).

[9] Dongwei Xu, Peter Zapol, G. Brian Stephenson, and Carol Thompson, "Kinetic Monte Carlo simulations of GaN homoepitaxy on c-and m-plane surfaces," The Journal of Chemical Physics **146**, 144702 (2017).
